# Supplementary material for: Navigation with QPHIL: Quantizing Planner for Hierarchical Implicit Q-Learning
Source: arXiv:2411.07760 source file (2024-11-12)
Supplement: Supplementary file 1 [file __additional_related.tex]

\section{Additional related work}

\textbf{Algorithms that may be useful for benchmarks:}

GCBC: Learning to Reach Goals via
Iterated Supervised Learning

WGCBC: RETHINKING GOAL-CONDITIONED SUPERVISED
LEARNING AND ITS CONNECTION TO OFFLINE RL \cite{yang2022rethinking}

GC-IQL: OFFLINE REINFORCEMENT LEARNING
WITH IMPLICIT Q-LEARNING

GC-POR: A Policy-Guided Imitation Approach for
Offline Reinforcement Learning

HGCBC: Relay Policy Learning: Solving Long-Horizon Tasks
via Imitation and Reinforcement Learning \cite{gupta2019relay}

TAP: Published as a conference paper at ICLR 2023
EFFICIENT PLANNING IN A COMPACT LATENT ACTION
SPACE

WT: Waypoint Transformer: Reinforcement Learning via
Supervised Learning with Intermediate Targets

HDMI: (diffusion + hierarchical planning)\cite{pmlr-v202-li23ad} 

VQ-VAE: Neural Discrete Representation Learning

HIPS: Hierarchical Imitation Learning with Vector Quantized Models

\textbf{Hierachical (Online) Goal Conditioned RL}:

Goal-conditioned reinforcement learning with imagined subgoals (2021): Au cours du training, on génère des subgoals sg pour aller de s à g via une politque high level, qui permet de guider l'apprentissage de la politique low level qui s'appuie sur l'action ag de s à sg pour aller de s à g, en online off-policy RL.

Feudal Reinforcement Learning(1992): Vieux papier pour la légacy, mais même idée générale.\cite{dayan1992feudal}

Hierarchical deep reinforcement learning (2016): Integrating temporal abstraction and intrinsic motivation: Version hierarchique du DQN pour le goal conditioned RL. \cite{kulkarni2016hierarchical}

Learning Multi-Level Hierarchies with Hindsight (2017):  Propose une approche hierarchique au goal conditioned RL online par le training en parallèle de k-politiques stackées, avec hindsight experience replay. \cite{levy2017learning}
